# Supplementary material for: A quantum phase transition in the one-dimensional water chain
Source: arXiv:2210.08124 source file (2022-11-10)
Supplement: Supplementary file 1 [file supp_info.pdf]

# Supplementary Material for: A quantum phase transition in the one-dimensional water chain

T. Serwatka,[1] R. G. Melko,[2,3] A. Burkov,[2,3] and P.-N. Roy[1,3]

[1] *Department of Chemistry, University of Waterloo, Ontario, N2L 3G1, Canada*
[2] *Department of Physics & Astronomy, University of Waterloo, Ontario, N2L 3G1, Canada*
[3] *Perimeter Institute for Theoretical Physics, Waterloo, Ontario N2L 2Y5, Canada*

## METHODS

The Hamiltonian of a chain of $N$ rotating water molecules interacting via pair-potentials is

$$H = \sum_{i=1}^{N} \left( A_e J_{a,i}^2 + B_e J_{b,i}^2 + C_e J_{c,i}^2 \right) + \sum_{ij} V(\Omega_i, \Omega_j; R), \tag{1}$$

where all molecules are fixed at their center-of mass at a water-water distance $R$. The rotational (kinetic) term contains the components of the total angular momentum along the principal axes $a, b, c$. For the rotational constant spectroscopic values of $A_e = 27.88\,\mathrm{cm}^{-1}$, $B_e = 14.51\,\mathrm{cm}^{-1}$ and $C_e = 9.29\,\mathrm{cm}^{-1}$ are employed [1]. The potential is approximated by a sum over pair-interactions, depending on the Euler angles $\Omega = \{\theta, \varphi, \chi\}$ of molecules at site $i$ and $j$ at a given water-water distance $R$. Since the quantum phase transitions occurs at rather large distances this pair-approximation is considered to be reasonable. For the pair-potential the very accurate accurate MB-pol potential [2, 3] is used. Both the bond length and angle of the single water molecules were fixed at 0.957 84 Å and 104.508°. The calculations are performed by a recently developed density-matrix renormalization group (DMRG) [4] approach whose details are explained in Ref. [5]. The calculations were performed using the iTensor software package [6].

In this study we present results calculated with a rotational basis of $j_{\max} = 1$ and by only considering nearest-neighbour interactions. This setting is sufficient to extract the physical behaviour of the system. Employing a larger basis, taking into account more pair-interactions or using a different water-water potential only shifts the critical point but it changes neither the qualitative results nor the critical exponents in accordance with a universal behaviour near a QPT .

The Schmidt spectrum $\{\lambda_l\}$ of the system's quantum state $|\Psi\rangle$ is obtained by a Schmidt decomposition:

$$|\Psi\rangle = \sum_l \sqrt{\lambda_l} |\phi_A^l\rangle \otimes |\phi_B^l\rangle \tag{2}$$

where the complete Hilbert space is decomposed in a bipartite tensor product $\mathcal{H} = \mathcal{H}_A \otimes \mathcal{H}_B$ with orthonormal sets $\{|\phi_A^l\rangle\}$ and $\{|\phi_B^l\rangle\}$ for region A and B, respectively. The Schmidt coefficients are nothing else but the eigenvalues of the reduced density matrices $\rho_A$ (and $\rho_B$) for the chosen partition and are directly connected to the von-Neumann entanglement entropy,

$$S_{\mathrm{vN}}(\rho_A) = -\mathrm{tr}(\rho_A \log \rho_A) \tag{3}$$

$$= -\sum_l \lambda_l \ln(\lambda_l). \tag{4}$$

**SYSTEM SIZE DEPENDENCE**

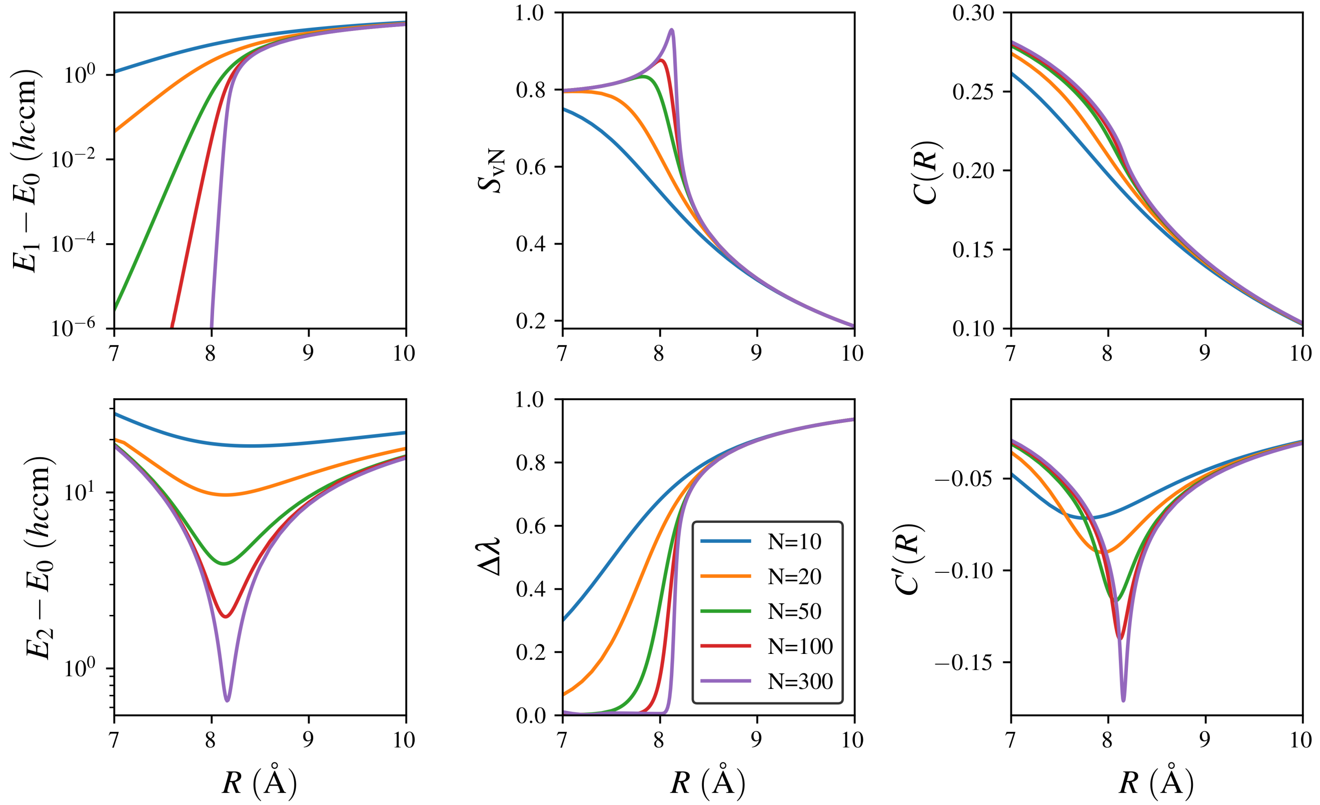


FIG. 1. Various properties calculated for chains of different number of chain sites. In all calculation only nearest-neighbour interactions were taken into account.

**J-CONVERGENCE AND POTENTIAL MODEL**

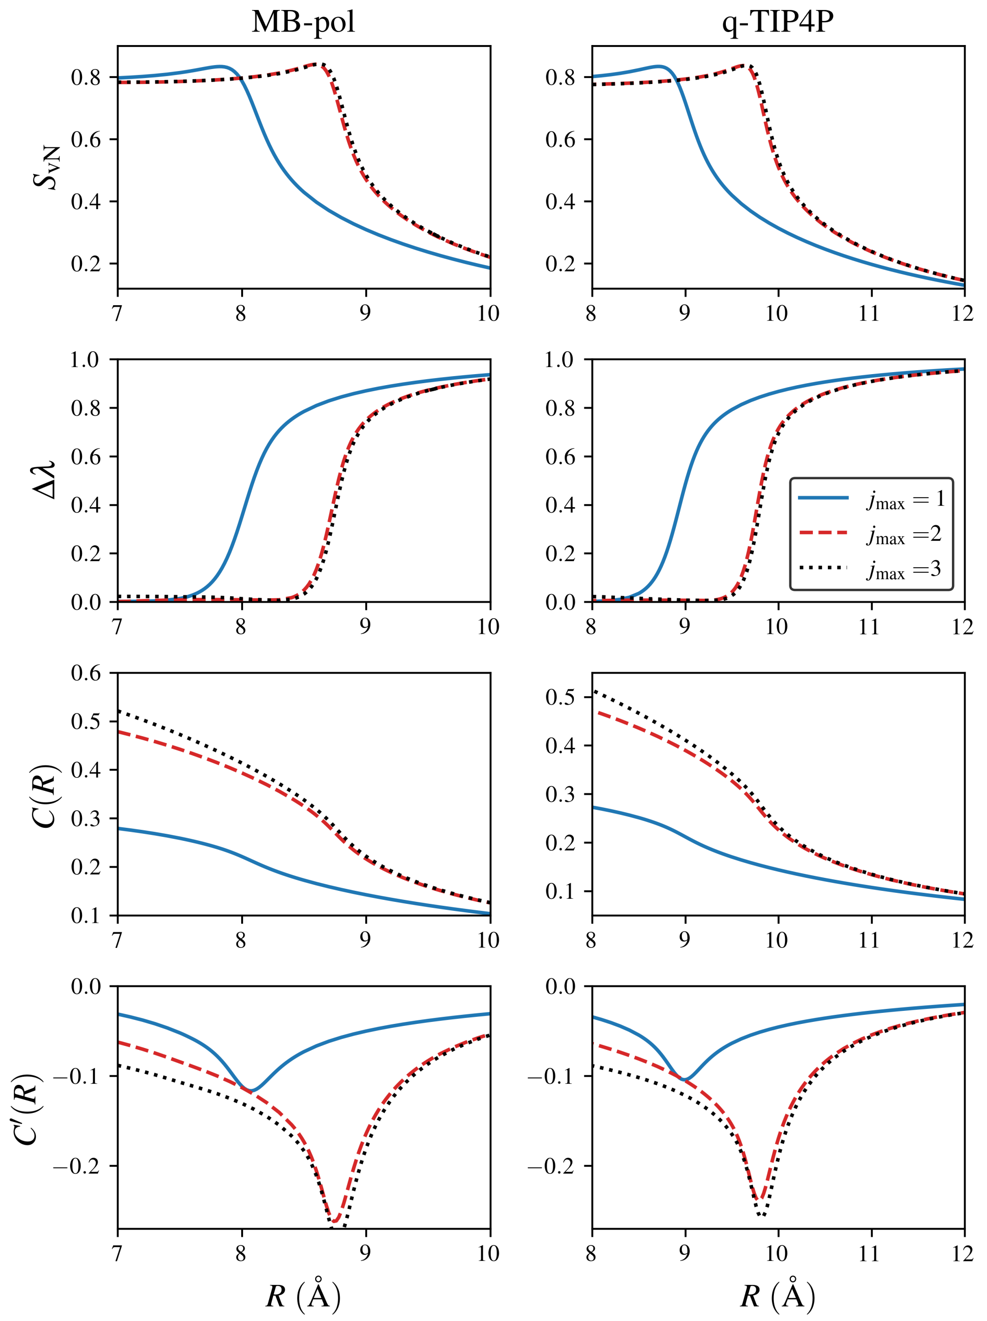


FIG. 2. Various properties calculated for different basis set sizes. Two different potential models, MB-pol (left half) and q-TIP4P (right half) employed. All results are calculated by considering only nearest-neighbour interactions for chains with $N = 50$.

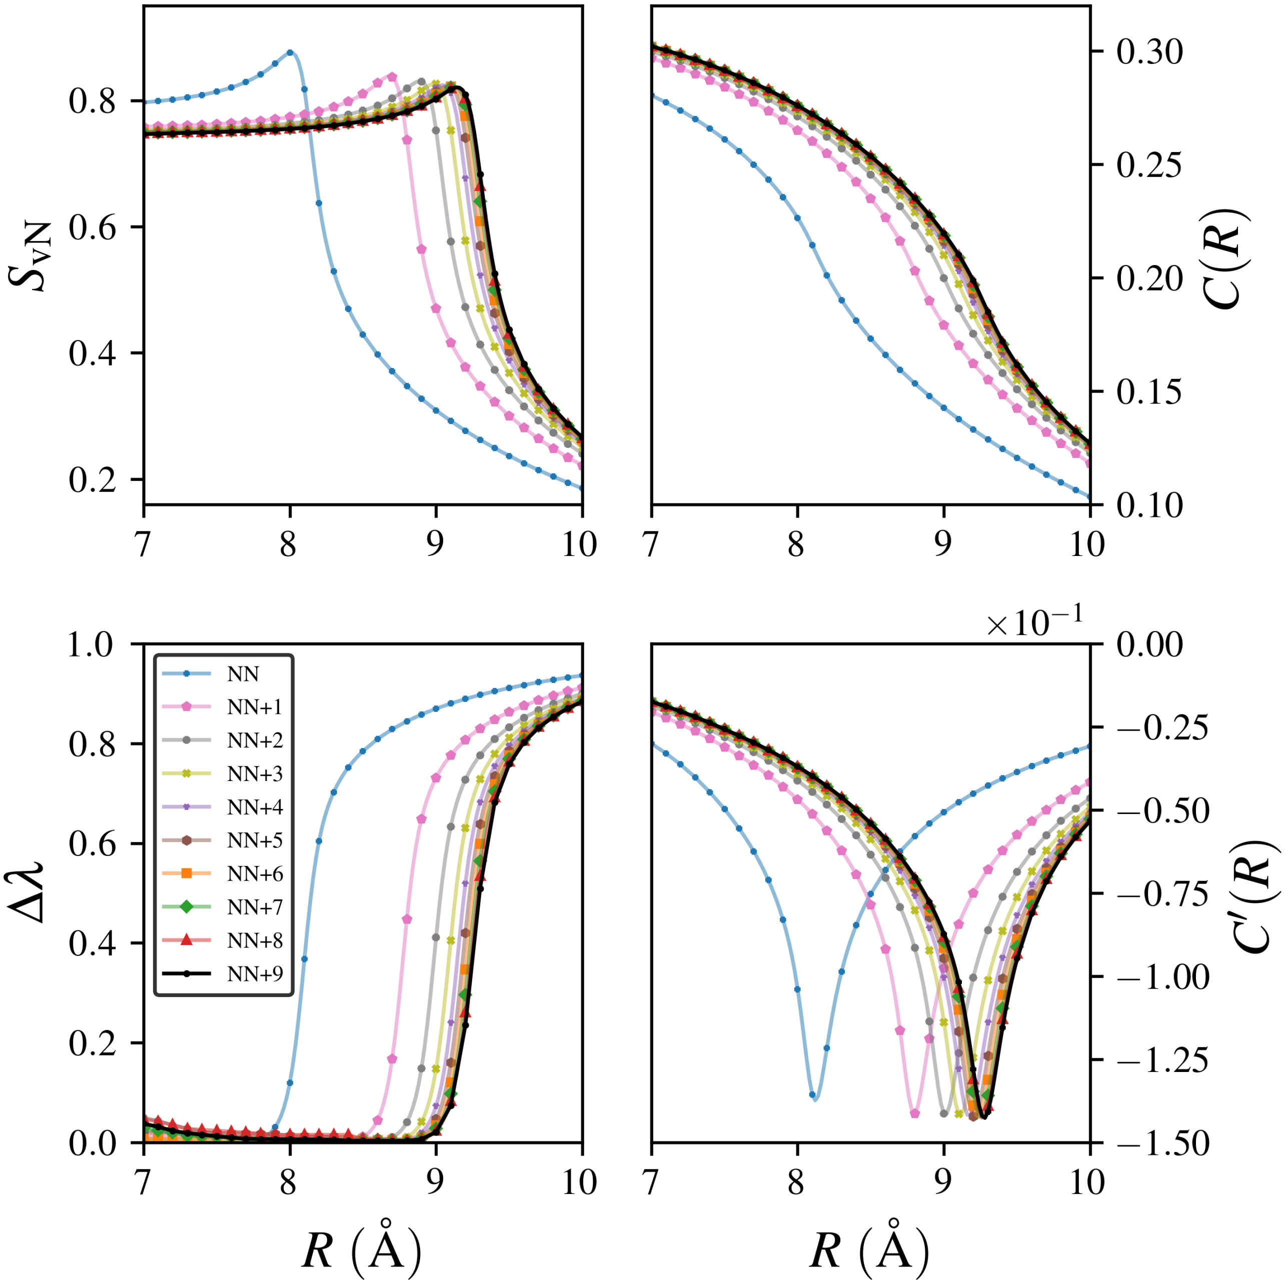


FIG. 3. Different properties calculated by taking into account nearest-neighbour (NN) interactions as well as pair- interactions beyond NN (NN+X). All results are calculated for chains with $N = 100$.

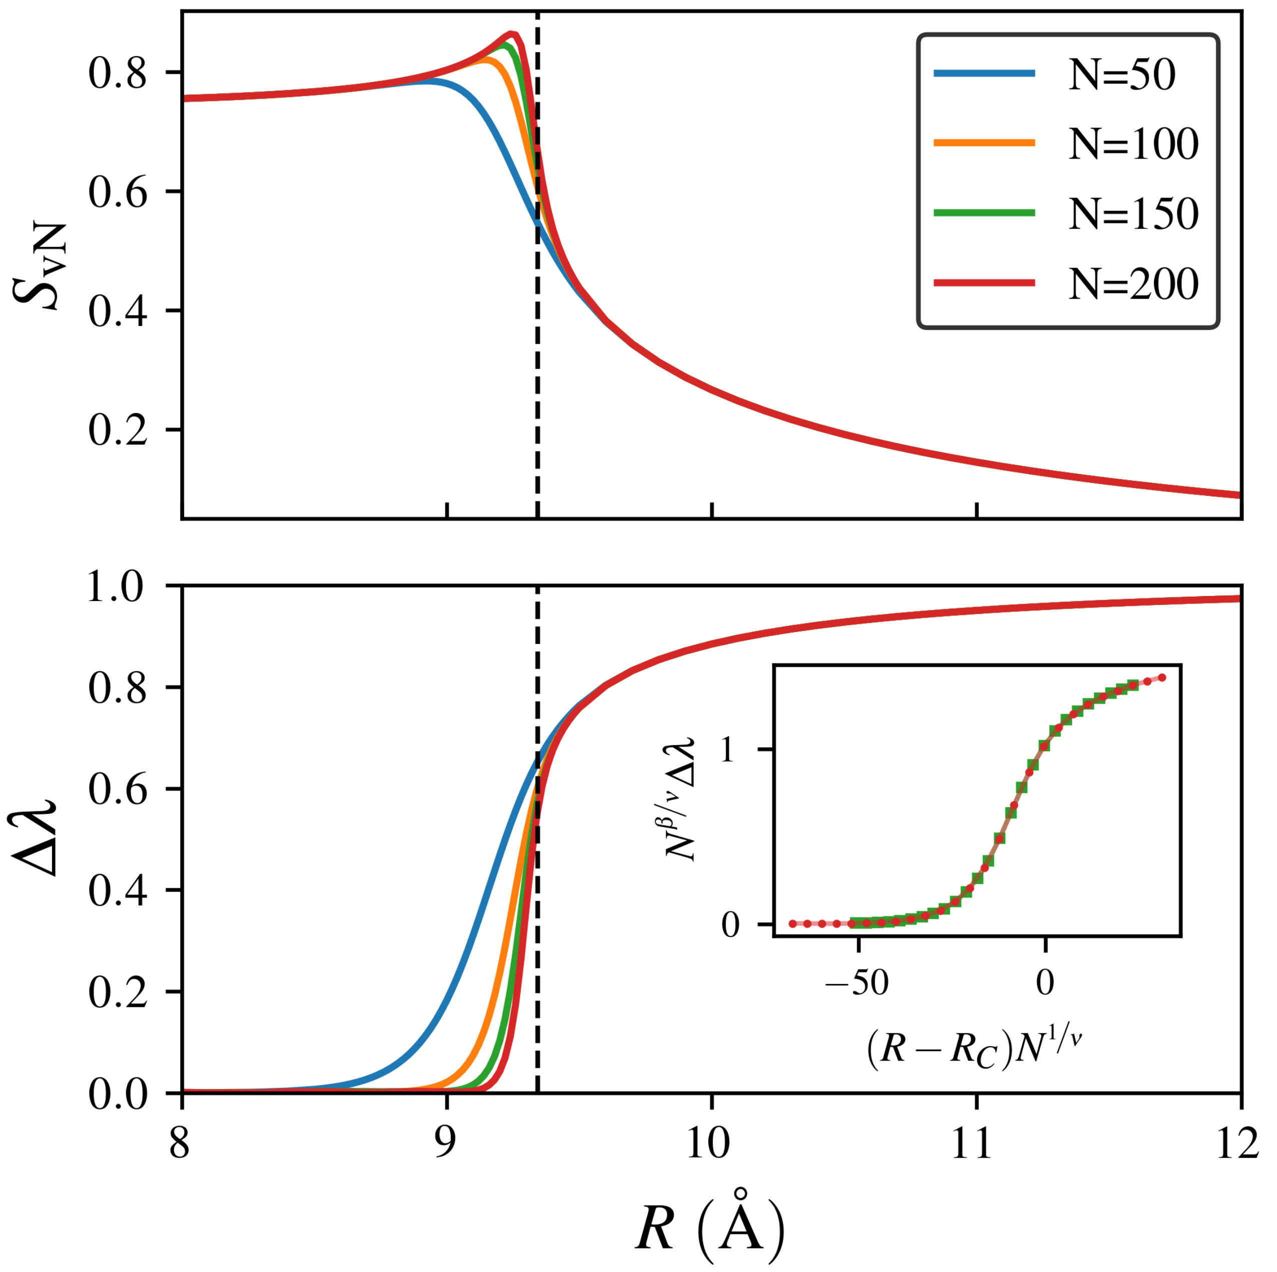


FIG. 4. Upper panel: von-Neumann entanglement entropy for chains of different numbers of chain sites. Lower panel: Schmidt gap for chains of different numbers of chain sites. Inset: Rescaled Schmidt gap for $N = 150$ and $N = 200$. The critical exponents are obtained by a finite-size scaling analysis which yields values of $\nu = 1.023 \pm 0.054$ and $\beta = 0.117 \pm 0.013$. The critical distance is indicated by the dashed vertical line. All calculation were done by considering all NN+9 interactions.

## REFERENCES


[1] Richard T Hall and Jerome M Dowling, "Pure rotational spectrum of water vapor," J. Chem. Phys. **47**, 2454–2461 (1967).

[2] Volodymyr Babin, Claude Leforestier, and Francesco Paesani, "Development of a "first principles" water potential with flexible monomers: Dimer potential energy surface, vrt spectrum, and second virial coefficient," J. Chem. Theory Comput. **9**, 5395 (2013).

[3] Volodymyr Babin, Gregory R Medders, and Francesco Paesani, "Development of a "first principles" water potential with flexible monomers. ii: Trimer potential energy surface, third virial coefficient, and small clusters," J. Chem. Theory Comput. **10**, 1599–1607 (2014).

[4] Steven R White, "Density matrix formulation for quantum renormalization groups," Phys. Rev. Lett **69**, 2863 (1992).

[5] Tobias Serwatka and Pierre-Nicholas Roy, "Ground state of asymmetric tops with dmrg: water in one dimension," J. Chem. Phys. (2022).

[6] Matthew Fishman, Steven R. White, and E. Miles Stoudenmire, "The ITensor software library for tensor network calculations," (2020), arXiv:2007.14822.
